# Supplementary material for: Seeking Specifications: The Case for Neuro-Symbolic Specification Synthesis
Source: arXiv:2504.21061 source file (2025-04-29)
Supplement: Supplementary file 1 [file appendix_programs_workshop.tex]

\section{Baseline Binary Search}
\label{BaselineBsearch}
Specification for Binary Search generated with the baseline prompt.

\begin{lstlisting}[style=cstyle]
/*@
  @ requires \valid(A + (0..9)) && \valid(&elem);
  @ ensures \result == 0 || \result == 1;
  @ assigns \nothing;
*/
int testme( int A[10], int elem) {
  int low, high, mid, ret ;
  low = 0 ;
  high = 9 ;
  ret = 0 ;
  /*@
    @ loop invariant high >= low;
    @ loop assigns low, high, mid, ret;
    @ loop variant high - low;
  */
  while( ( high > low ) )
    { mid = (low + high) / 2 ;

      if( elem == A[mid] )
         ret = 1;
      if( elem > A[mid] )
        low = mid + 1 ;
      else
        high = mid - 1;
    }
  mid = (low + high) / 2 ;

  if( ( ret != 1)  && ( elem == A[mid]) )
    ret = 1;

  return ret ;
}
\end{lstlisting}

\section{Preliminary Baseline Binary Search}
\label{PrelimBaselineBsearch}
Specification generated with an earlier verison of GPT-4

\begin{lstlisting}[style=cstyle]
/*@
  @ requires \valid(A + (0..9));
  @ requires \forall integer i, j; 0 <= i < j < 10 ==> A[i] <= A[j]; // Array is sorted
  @ assigns \nothing;
  @ ensures \result == 1 <==> \exists integer i; 0 <= i < 10 && A[i] == elem;
*/
int testme( int A[10], int elem) {
  int low, high, mid, ret ;

  /*@
    @ assigns low;
  */
  low = 0 ;

  /*@
    @ assigns high;
  */
  //@assert true;
  high = 9 ;

  /*@
    @ assigns ret;
  */
  ret = 0 ;

  /*@
    @ loop invariant 0 <= low <= high <= 9;
    @ loop assigns low, high, mid, ret;
    @ loop variant high - low;
  */
  while( ( high > low ) )
    {
      /*@
        @ assigns mid;
      */
      mid = (low + high) / 2 ;

      /*@
        @ assigns ret;
      */
      if( elem == A[mid] )
         ret = 1;

      /*@
        @ assigns low;
      */
      if( elem > A[mid] )
        low = mid + 1 ;
      else
      /*@
        @ assigns high;
      */
        high = mid - 1;
    }

  /*@
    @ assigns mid;
  */
  mid = (low + high) / 2 ;

  /*@
    @ assigns ret;
  */
  if( ( ret != 1)  && ( elem == A[mid]) )
    ret = 1;

  /*@
    @ assigns \nothing;
  */
  return ret ;
}
\end{lstlisting}

\section{LabelsTritype Augmented with an Eva Report}
\label{LabelsTritypeEVA}
LabelsTritype is a version of Tritype that is meant to test the labeling feature of Pathcrawler. The following is a specification generated for LabelsTritype with an Eva report added.

\begin{lstlisting}[style=cstyle]
/*@ requires Side1 > 0 && Side2 > 0 && Side3 > 0;
  @ ensures \result >= 1 && \result <= 4;
  @ assigns \nothing;*/
int testme (int Side1, int Side2, int Side3){
   int triOut;
   /*@ assert Side1 <= 2147483647 && Side2 <= 2147483647 && Side3 <= 2147483647; */
   if (Side1 <= 0 || Side2 <= 0 || Side3 <= 0)
   {
      triOut = 4;
      return (triOut);
   }
   triOut = 0;
   if (Side1 == Side2){ triOut = triOut + 1;}
   if (Side1 == Side3){ triOut = triOut + 2;}
   if (Side2 == Side3){triOut = triOut + 3;}
   if (triOut == 0)
   {
     /*@ assert Side1+Side2 <= 2147483647 && Side1+Side3 <= 2147483647 && Side2+Side3 <= 2147483647; */

     if (Side1+Side2 <= Side3 || Side2+Side3 <= Side1 || Side1+Side3 <= Side2){triOut = 4;}
     else{triOut = 1;}
     return (triOut);
   }
   if (triOut > 3){triOut = 3;}
   else{
     /*@ assert Side1+Side2 <= 2147483647 && Side1+Side3 <= 2147483647 && Side2+Side3 <= 2147483647; */
     if (triOut == 1 && Side1+Side2 > Side3){triOut = 2;}
     else{
       if (triOut == 2 && Side1+Side3 > Side2){triOut = 2;}
       else{
         pathcrawler_label(triOut == 3);
         pathcrawler_label(triOut != 3);
         pathcrawler_label(Side2+Side3 > Side1);
         pathcrawler_label(Side2+Side3 <= Side1);
         if (triOut == 3 && Side2+Side3 > Side1){triOut = 2;}
         else{triOut = 4;}
       }
     }
   }
   return (triOut);
}
\end{lstlisting}

The EVA report provided to the prompt:
\begin{lstlisting}[style=cotstyle]
[kernel] Parsing temp_files/tmpifalg4bf/eva_temp.c (with preprocessing)
[kernel:typing:implicit-function-declaration] temp_files/tmpifalg4bf/eva_temp.c:20: Warning:
  Calling undeclared function pathcrawler_label. Old style K&R code?
[eva] Option -eva-precision 7 detected, automatic configuration of the analysis:
  option -eva-min-loop-unroll set to 0 (default value).
  option -eva-auto-loop-unroll set to 256.
  option -eva-widening-delay set to 4.
  option -eva-partition-history set to 1.
  option -eva-slevel set to 250.
  option -eva-ilevel set to 128.
  option -eva-plevel set to 300.
  option -eva-subdivide-non-linear set to 140.
  option -eva-remove-redundant-alarms set to true (default value).
  option -eva-domains set to 'cvalue,equality,gauges,octagon,symbolic-locations'.
  option -eva-split-return set to 'auto'.
  option -eva-equality-through-calls set to 'formals' (default value).
  option -eva-octagon-through-calls set to true.
[eva] Splitting return states on:
[eva] Analyzing an incomplete application starting at testme
[eva] Computing initial state
[eva] Initial state computed
[eva:initial-state] Values of globals at initialization

[kernel:annot:missing-spec] temp_files/tmpifalg4bf/eva_temp.c:20: Warning:
  Neither code nor specification for function pathcrawler_label, generating default assigns from the prototype
[eva] using specification for function pathcrawler_label
[eva:alarm] temp_files/tmpifalg4bf/eva_temp.c:67: Warning:
  signed overflow. assert Side1 + Side2 <= 2147483647;
[eva:alarm] temp_files/tmpifalg4bf/eva_temp.c:69: Warning:
  signed overflow. assert Side1 + Side3 <= 2147483647;
[eva:alarm] temp_files/tmpifalg4bf/eva_temp.c:71: Warning:
  signed overflow. assert Side2 + Side3 <= 2147483647;
[eva:alarm] temp_files/tmpifalg4bf/eva_temp.c:100: Warning:
  signed overflow. assert Side1 + Side2 <= 2147483647;
[eva:alarm] temp_files/tmpifalg4bf/eva_temp.c:112: Warning:
  signed overflow. assert Side1 + Side3 <= 2147483647;
[eva:alarm] temp_files/tmpifalg4bf/eva_temp.c:124: Warning:
  signed overflow. assert Side2 + Side3 <= 2147483647;
[eva] done for function testme
[eva] ====== VALUES COMPUTED ======
[eva:final-states] Values at end of function testme:
  triOut in {1; 2; 3; 4}
  __retres in {1; 2; 3; 4}
[eva:summary] ====== ANALYSIS SUMMARY ======
  ------------------------------
  1 function analyzed (out of 1): 100% coverage.
  In this function, 73 statements reached (out of 73): 100% coverage.
  ------------------------------
  Some errors and warnings have been raised during the analysis:
    by the Eva analyzer:      0 errors    0 warnings
    by the Frama-C kernel:    0 errors    2 warnings
  ------------------------------
  6 alarms generated by the analysis:
       6 integer overflows
  -------------------------------
  No logical properties have been reached by the analysis.
\end{lstlisting}

\section{Mutated Levenshtein}
\label{code:code_mutated_levenshtein}
Mutated Levenshtein distance algorithm with typos highlighted in red
\begin{lstlisting}[style=cstyle]
#include <string.h>

/*@ requires \true;
  @ ensures \result <= x && \result <= y && \result <= z;
  @ assigns \nothing;
*/
int min(int x, int y, int z) {
    if (x < y) return (x < z) ? x : z;
    else return (y < z) ? y : z;
}
/*@ requires \valid(s1) && \valid(s2);
  @ ensures \result >= 0;
  @ assigns \nothing;
*/
int levenshtein(char *s1, char *s2) {
    int len1 = strlen(s1), len2 = strlen(s2);
    int matrix[len1 + 1][len2 + 1];

    /*@ loop invariant 0 <= x <= len1;
      @ loop assigns matrix[0][0 .. len1];
    */
    for (int x = 0; x <= len1; x++) @@matrix[0][x]@@ = x;

    /*@ loop invariant 0 <= y <= len2;
      @ loop assigns matrix[0 .. len2][0];
    */
    for (int y = 0; y <= len2; y++) @@matrix[y][0]@@ = y;
    /*@ loop invariant 1 <= x <= len1;
      @ loop assigns matrix[1 .. len1][1 .. len2];
    */
    for (int x = 1; x <= len1; x++) {
        /*@ loop invariant 1 <= y <= len2;
          @ loop assigns matrix[x][1 .. len2];
        */
        for (int y = 1; y <= len2; y++) {
            int cost = (s1[x - 1] == s2[y - 1]) ? 0 : 1;
            matrix[x][y] = min(matrix[x - 1][y] + 1, matrix[x][y - 1] + 1, matrix[x - 1][y - 1] + cost);
        }
    }
    return matrix[len1][len2];
}
\end{lstlisting}

\section{BugKPath Baseline}
\label{code:bugkpath_baseline}
\begin{lstlisting}[style=cstyle]
/*@ requires \valid(msg + (0 .. len-1)) && \valid(buffer + (0 .. BUFSZ-1));
  @ requires len >= 0;
  @ assigns buffer[0 .. BUFSZ-1];
  @*/
void testme (char *msg, int len, char *buffer)
{
  int i;
  int j;
  int limit = BUFSZ - 1;
  /*@ loop invariant 0 <= i <= len;
    @ loop variant len - i;
    @*/
  for (i = 0; i < len; ) {
    /*@ loop invariant 0 <= j <= limit;
      @ loop assigns buffer[0 .. limit];
      @ loop variant limit - j;
      @*/
    for (j = 0; i < len && j < limit; ){
    ...
    }
  }
}
\end{lstlisting}

\section{Apache Pathcrawler}
\label{ApachePC}
Specification generated for the Apache program with Pathcrawler input/output pairs as additional context

\begin{lstlisting}[style=cstyle]
#include "apache.h"

/*@
  @ requires \valid(s);
  @ ensures \result >= 0;
*/
unsigned mystrlen(char *s)
{
  int i;
  i = 0;
  /*@
    @ loop invariant \valid(s+i);
    @ loop assigns i;
  */
  while (s[i] != EOS)
    ++i;
  return i;
}

/*@
  @ requires \valid(s1) && \valid(s2) && n >= 0;
  @ ensures \result <= 0 || \result == 0 || \result > 0;
*/
int mystrncmp (const char *s1, const char *s2, int n)
{
  int i;
  int retval;
  i = 0;
  /*@
    @ loop invariant \valid(s1+i) && \valid(s2+i) && i <= n;
    @ loop assigns i, retval;
  */
  do {
    retval = s1[i] - s2[i];
    if (i >= n-1) return retval;
    if (retval != 0) return retval;
    if (s1[i] == EOS) return 0;
    i++;
  } while (1);
}
/*@
  @ requires scheme >= 0 && \valid(uri);
  @ assigns uri[0..TOKEN_SZ];
*/
void testme (char *uri, int scheme)
{
  int cp;
  int c,i;
  char LDAP[5]={"ldap"};
  char *token[TOKEN_SZ];
  if (scheme == 0
      || mystrlen(uri) < scheme) {
    return;
  }
  cp = scheme;

  if (uri[cp-1] == '/') {

    while (uri[cp] != EOS
           && uri[cp] != '/') {
      ++cp;
    }
    if (uri[cp] == EOS || uri[cp+1] == EOS) return;
    ++cp;
    scheme = cp;
    if (mystrncmp(uri, LDAP, LDAP_SZ) == 0) {
      c = 0;
      token[0] = uri;

      while (uri[cp] != EOS
             && c < TOKEN_SZ) {
        if (uri[cp] == '?') {
          ++c;
          token[c] = uri + cp + 1;
          uri[cp] = EOS;
        }
        ++cp;
      }
      return;
    }
  }
  return;
}
\end{lstlisting}

The Pathcrawler Input/Output pairs provided. Notice how no output is provided. Since Apache is a void function with side-effects, the input output pairs say nothing about the program.

\begin{lstlisting}
input_scheme,input_uri[0],...,input_uri[14],output,verdict
1,47,47,0,0,0,0,0,0,0,0,0,0,0,0,0,,unknown
1,47,58,0,0,0,0,0,0,0,0,0,0,0,0,0,,unknown
2,108,47,47,47,0,0,0,0,0,0,0,0,0,0,0,,unknown
1,47,0,0,0,0,0,0,0,0,0,0,0,0,0,0,,unknown
5,108,100,97,112,47,47,63,0,0,0,0,0,0,0,0,0,unknown
5,108,100,97,112,47,47,63,47,63,63,0,0,0,0,0,,no_extra_coverage
5,108,100,97,112,47,47,63,63,63,0,0,0,0,0,0,,no_extra_coverage
0,0,0,0,0,0,0,0,0,0,0,0,0,0,0,0,,unknown
422214939,0,0,0,0,0,0,0,0,0,0,0,0,0,0,0,,unknown
1,47,47,47,0,0,0,0,0,0,0,0,0,0,0,0,,unknown
1,58,0,0,0,0,0,0,0,0,0,0,0,0,0,0,,unknown
5,108,100,97,112,47,47,63,63,63,47,0,0,0,0,0,,unknown
5,108,100,97,112,47,47,63,63,47,63,0,0,0,0,0,,no_extra_coverage
4,108,100,97,47,47,47,0,0,0,0,0,0,0,0,0,,unknown
5,108,100,97,112,47,47,47,0,0,0,0,0,0,0,0,,unknown
422214939,47,0,0,0,0,0,0,0,0,0,0,0,0,0,0,,unknown
5,108,100,97,112,47,47,47,63,63,63,0,0,0,0,0,,no_extra_coverage%
\end{lstlisting}

% \section{Mutated Tritype}
% \label{code:mutated_tritype}
% Mutated Tritype with typos highlighted in red
% \label{code:mutated_tritype}
% \begin{lstlisting}[style=cstyle]
% /*@
%   @ requires i >= 0 && j >= 0 && k >= 0;
%   @ assigns \nothing;
%   @ behavior not_triangle:
%   @   assumes i == 0 || j == 0 || k == 0 || i+j <= k || j+k <= i || i+k <= j;
%   @   ensures \result == 4;
%   @ behavior equilateral_triangle:
%   @   assumes i != 0 && j != 0 && k != 0 && i == j && j == k;
%   @   ensures \result == 3;
%   @ behavior isosceles_triangle:
%   @   assumes i != 0 && j != 0 && k != 0 && ((i == j && j != k) || (i != j && j == k) || (i == k && j != k));
%   @   ensures \result == 2;
%   @ behavior scalene_triangle:
%   @   assumes i != 0 && j != 0 && k != 0 && i != j && j != k && i != k && i+j > k && j+k > i && i+k > j;
%   @   ensures \result == 1;
% */
% int tritype(int i, int j, int k){
%   int type_code;
%   if ((i == 0) || (j == 0) || (k == 0)) type_code = 4;
%   else {
%     type_code = 0;
%     if (i == j) type_code = type_code + 1;
%     if (i == k) type_code = type_code + 2;
%     if (j == k) type_code = type_code + 3;
%     if (type_code == 0){
%       if ((i+j <= k) || @@(i+k <= i)@@ || (i+k <= j))
% 	type_code = 4;
%       else
% 	type_code = 1;
%       }
%     else if (type_code > 3) type_code = 3;
%     else if ((type_code == 1) && (i+j > k)) type_code = 2;
%     else if ((type_code == 2) && @@(i+k > j))@@ type_code = 2;
%     else if ((type_code == 3) && (i+k > i)) type_code = 2;
%     else type_code = 4;
%     }
%   return type_code;
% }
% \end{lstlisting}
