# Supplementary material for: Seeking Specifications: The Case for Neuro-Symbolic Specification Synthesis
Source: arXiv:2504.21061 source file (2025-04-29)
Supplement: Supplementary file 2 [file appendix_prompts_shortened.tex]

\section{Prompts}
\begin{lstlisting}[style=cotstyle]
You are a LLM that takes the following inputs and returns a C program annotated with ACSL annotations.
Inputs:
1. A C program with no ACSL annotations
GOALS:
1. Describe any abstract properties that could be represented as ACSL annotations
2. Generate ACSL annotations based on your analysis of the program
3. Returning a program with no annotation is not a valid solution
4. Do not edit the C code, only add annotations
5. Make sure to describe your thought process behind the annotations
6. Do not skip any code in the returned solution to make it shorter.
7. If you break any of these rules then my family will disown me.
...
START OF INPUT:
{program}
\end{lstlisting}
\label{PromptBaseline}

\begin{lstlisting}[style=cotstyle]
2. Analyze the pathcrawler CSV and describe any patterns that you see that could help you understand the behaviors of the program based on given input/output pairs
...
4. Generate ACSL annotations based on your analysis of the program and take special account of the properties described when analyzing the Pathcrawler CSV file
...
PathCrawler Output:
{csv}
\end{lstlisting}
\label{PromptPC}

\begin{lstlisting}[style=cotstyle]
2. Analyze the Eva report and describe how the results could be used in generating ACSL annotations
3. Generate ACSL annotations based on your analysis of the program and take special account of the properties described when analyzing the Eva report
...
Eva Report:
{eva}
\end{lstlisting}
\label{PromptEVA}
